# Supplementary material for: Low-Noise YBa$_2$Cu$_3$O$_7$ NanoSQUIDs for Performing Magnetization-Reversal Measurements on Magnetic Nanoparticles
Source: arXiv:1503.06090 source file (2015-03-20)
Supplement: Supplementary file 1 [file Supplement_YBCOnanoSQUIDs.pdf]

# Supplementary Information for Low-Noise $YBa_2Cu_3O_7$ NanoSQUIDs for Performing Magnetization-Reversal Measurements on Magnetic Nanoparticles

T. Schwarz,[1] R. Wölbing,[1] C. F. Reiche,[2] B. Müller,[1]
M. J. Martínez-Pérez,[1] T. Mühl,[2] B. Büchner,[2] R. Kleiner,[1] and D. Koelle[1]

[1] *Physikalisches Institut – Experimentalphysik II and Center for Collective Quantum Phenomena in LISA*$^+$*, Universität Tübingen, Auf der Morgenstelle 14, D-72076 Tübingen, Germany*

[2] *Leibniz Institute for Solid State and Materials Research IFW Dresden, Helmholtzstr. 20, 01069 Dresden, Germany*

(Dated: March 20, 2015)

## I. CHARACTERIZATION OF SQUID-2

SQUID-2 was characterized in an electrically and magnetically shielded setup, with the sample mounted in vacuum (or in He gas) on a temperature-controlled cryostage. This enabled us to characterize electric transport and noise properties at variable temperature $T$, with a $T$ stability of $\sim 1\,$mK [1].

Figure 1 shows data of electric transport properties and flux noise of SQUID-2, measured at $T = 5.3\,$K. Figure 1(a) shows current-voltage-characteristics (IVCs) for modulation current $I_{\rm mod} = 0$ and two values of $I_{\rm mod}$, corresponding to maximum and minimum critical current. The IVCs are slightly hysteretic with maximum critical current $I_{\rm c} = 311\,\mu$A and normal state resistance $R_{\rm N} = 2.5\,\Omega$, which yields a characteristic voltage $V_{\rm c} \equiv I_{\rm c}R_{\rm N} = 0.78\,$mV. The inset of Fig. 1(a) shows the modulation of the critical current $I_{\rm c}(I_{\rm mod})$. From the modulation period, we find for the magnetic flux $\Phi$ coupled to the SQUID by $I_{\rm mod}$ the mutual inductance $M = \Phi/I_{\rm mod} = 0.8\,\Phi_0/$mA $= 1.66\,$pH. From resistively and capacitively shunted junction (RCSJ) simulations [2] of the $I_{\rm c}(I_{\rm mod})$ characteristics [cf. inset of Fig. 1(a)] we obtain for the screening parameter $\beta_L = 2I_0L/\Phi_0 = 0.94$ (with $I_0 = I_{\rm c}/2$), which yields a SQUID inductance $L = 6.3\,$pH. We do find good agreement between the measured and simulated $I_{\rm c}(I_{\rm mod})$ characteristics if we include an inductance asymmetry $\alpha_L \equiv (L_2 - L_1)/(L_2 + L_1) = 0.83$ ($L_1$ and $L_2$ are the inductances of the two SQUID arms) and a critical current asymmetry $\alpha_I \equiv (I_{0,2} - I_{0,1})/(I_{0,2} + I_{0,1}) = 0.30$; $I_{0,1}$ and $I_{0,2}$ are the critical currents of the Josephson junctions 1 and 2, respectively, intersecting the SQUID loop. These asymmetries are caused by asymmetric biasing of the SQUID and by asymmetries of the device itself.

$V(I_{\rm mod})$ is plotted in Fig. 1(b) for different bias currents. The transfer function, i.e. the maximum value of $\partial V/\partial\Phi$, in the non-hysteretic regime is $V_\Phi \approx 1.7\,$mV$/\Phi_0$.

Fig. 1(c) shows the rms spectral density of flux noise $S_\Phi^{1/2}(f)$ of SQUID-2. This measurement was performed open loop (in dc bias mode) with a Nb dc SQUID (at $T = 4.2\,K$) as a voltage preamplifier, i.e. in 2-stage configuration, with a $\sim 700\,$kHz bandwidth. As for SQUID-1 (see main text), we find dominating $f$-dependent noise, with a noise power which scales very roughly as $S_\Phi \propto 1/f$.

Figure 2 shows rms flux noise spectra of SQUID-2 measured with direct readout in flux locked loop (FLL), with

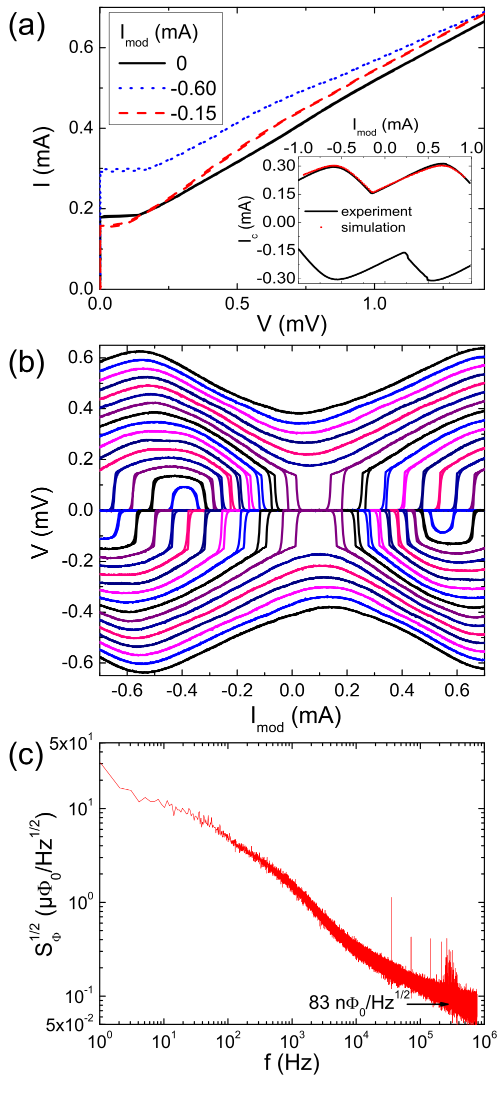


FIG. 1. Characteristics of SQUID-2 at $T = 5.3\,$K. (a) IVCs for three different values of $I_{\rm mod}$, including flux bias ($I_{\rm mod}$) values which yield maximum and minimum critical current. Inset: measured $I_{\rm c}(I_{\rm mod})$ together with numerical simulation results. (b) $V(I_{\rm mod})$ for bias currents $|I| = 175\ldots400\,\mu$A (in $15\,\mu$A steps). (c) rms spectral density of flux noise, measured open loop (dc bias) in 2-stage configuration. Arrow indicates upper limit for measured white noise at $\sim 700\,$kHz.

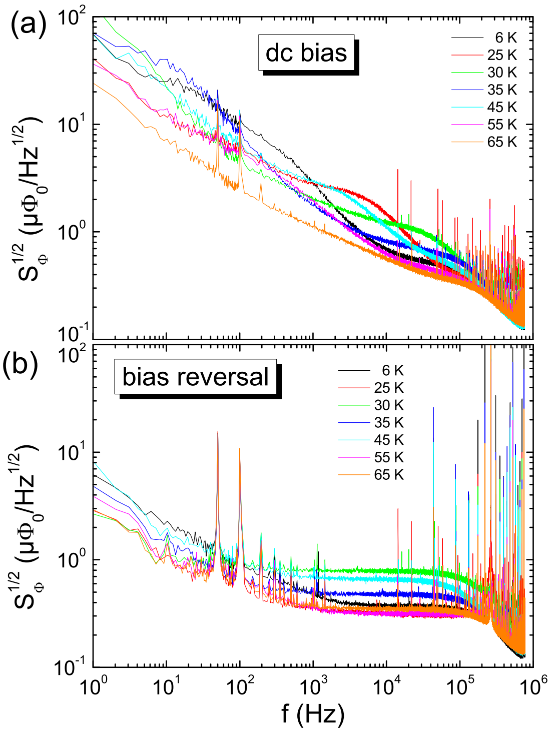


FIG. 2. rms spectral density of flux noise for SQUID-2, measured in FLL mode at different temperatures from 6 K to 65 K. (a) dc bias mode (b) bias reversal mode ($f_{\rm br}$ = 260 kHz).

$\sim$ 500 kHz bandwidth, in dc bias and bias reversal mode [3] for temperatures $T$ ranging from 6 K to 65 K. For all data measured with dc bias [cf. Fig. 2(a)], we find $f$-dependent excess noise up to the cutoff frequency of the readout electronics. The flux noise $S_\Phi$ scales roughly as $1/f$, and for different $T$, the rms flux noise does not differ by more than about a factor of five, and does not show any systematic $T$-dependence.

Similar to SQUID-1 (cf. main text), in bias reversal mode [cf. Fig. 2(b)] the $f$-dependent excess noise above $\sim$ 1 kHz is suppressed. The remaining low-$f$ excess flux noise observed in bias reversal mode roughly scales as $S_\Phi \propto 1/f$ for all values of $T$, again without any systematic $T$-dependence.

## II. CHARACTERIZATION OF SQUID-3

Figure 3 shows electric transport and flux noise data for SQUID-3, taken in the magnetically and electrically shielded low-field setup at $T$ = 4.2 K, as described in the main text. The IVC shown in Fig. 3(a) is non-hysteretic, with $I_{\rm c}$ = 69 $\mu$A and $R_{\rm N}$ = 2.3 $\Omega$, which yields $V_{\rm c}$ = 0.16 mV. The inset shows $I_{\rm c}(I_{\rm mod})$, from which we obtain the mutual inductance $M = \Phi/I_{\rm mod}$ = 3.3 $\Phi_0$/mA. From the modulation depth of $I_{\rm c}(I_{\rm mod})$ we determine $\beta_L = 0.95$. With the measured $I_{\rm c}$, this yields a SQUID inductance $L$ = 28 pH. The bumps in the IVC at $V_{\rm res} \approx \pm 0.28$ mV, can be attributed to an $LC$ resonance. From the relation $V_{\rm res}/I_{\rm c}R_{\rm N} = (\frac{\pi}{2}\beta_C\beta_L)^{-1/2}$ [2] we determine the Stewart-McCumber parameter for the GBJJs as $\beta_C \approx 0.22$.

Figure 3(b) shows $V(I_{\rm mod})$ curves for different bias currents, yielding a transfer function $V_\Phi$ = 0.65 mV/$\Phi_0$ at the optimum bias point, at which noise spectra have been taken ($I$ = 54 $\mu$A). Figure 3(c) shows the rms spectral density of flux noise $S_\Phi^{1/2}(f)$ for SQUID-3, measured in direct readout FLL mode up to $f$ = 100 kHz. For comparison, the bottom trace shows the background noise from the readout electronics $S_\Phi^{1/2} \approx 1.45\,\mu\Phi_0/{\rm Hz}^{1/2}$. For

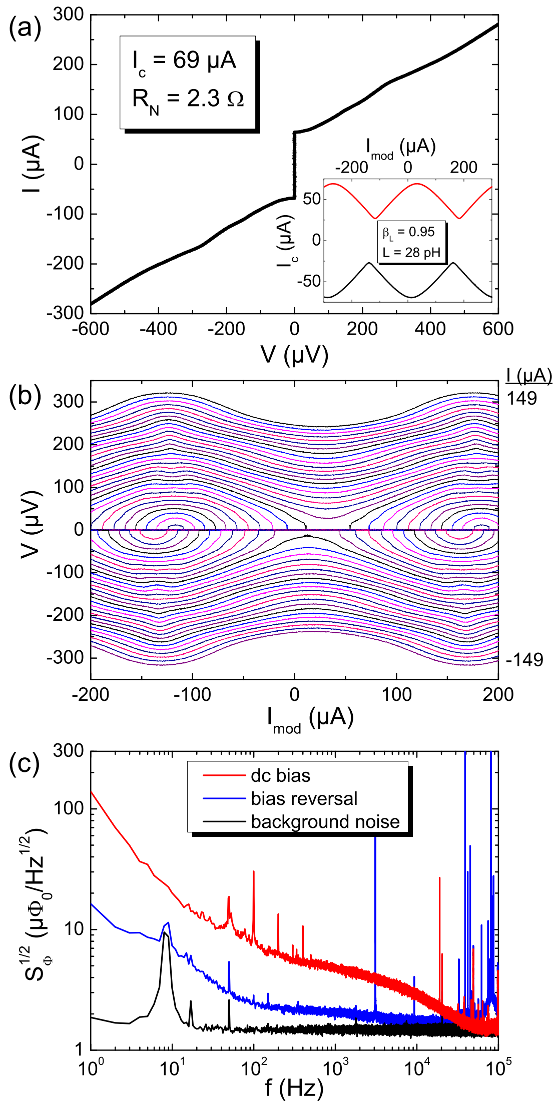


FIG. 3. Electric transport and noise characteristics of SQUID-3. (a) IVC of SQUID-3 for flux bias ($I_{\rm mod}$) which yields maximum critical current. Inset shows $I_{\rm c}(I_{\rm mod})$ curves for positive and negative current bias. (b) Voltage $V$ vs modulation current $I_{\rm mod}$ for bias currents between $I = \pm 149\,\mu$A (step width $\Delta I \approx 4\,\mu$A). (c) Rms spectral density of flux noise measured in FLL with dc bias and bias reversal mode ($f_{\rm br}$ = 260 kHz). The lower trace shows the background noise of the readout electronics.

$f \lesssim 40\,\text{kHz}$, we find $f$-dependent flux noise. For larger $f$, the noise is limited by the electronics background noise. Hence, we can only give an upper limit of the white rms flux noise of SQUID-3 as $S_{\Phi,\text{w}}^{1/2} < 1.45\,\mu\Phi_0/\text{Hz}^{1/2}$. With bias reversal (at $f_{\text{br}} = 81\,\text{kHz}$), the $f$-dependent excess noise is clearly reduced. Still, we obtain with decreasing $f$ a slight increase in rms flux noise up to $\sim 2.4\,\mu\Phi_0/\text{Hz}^{1/2}$ at 100 Hz. Below 100 Hz SQUID-3 shows approximately $1/f$ noise, i.e. an increase in $S_\Phi^{1/2}$ to $\sim 16\,\mu\Phi_0/\text{Hz}^{1/2}$ at 1 Hz.

## III. ANALYSIS OF NOISE SPECTRA OF SQUID-1

For a more detailed analysis of the measured spectral density of equivalent flux noise power $S_\Phi(f)$ for SQUID-1, we applied an algorithm [4] to decompose the noise spectra into a sum of Lorentzians $F_i(f) = F_{0,i}/[1 + (f/f_{\text{c},i})^2]$ plus a $1/f^2$ spectrum $F_\text{s}(f) = F_\text{s}(1\,\text{Hz})/(f^2/\text{Hz}^2)$ (i.e. one or more Lorentzians with characteristic frequencies $f_\text{c}$ well below 1 Hz) plus a white noise contribution $F_\text{w}$. This means, the measured spectra are fitted by $F(f) = F_\text{w} + F_\text{s} + \sum_i F_i$

Figure 4 shows the fit $F_{\text{op}}^{1/2}(f)$ to the spectrum measured open loop (dc bias) [cf. Fig. 3(a) in the main text.]. This yields an rms white noise level $F_{\text{w,op}}^{1/2} = 45\,\text{n}\Phi_0/\text{Hz}^{1/2}$, a 1 Hz noise $F_{\text{s,op}}^{1/2} = 84\,\mu\Phi_0/\text{Hz}^{1/2}$ from $F_{\text{s,op}}$ plus 16 Lorentzians with characteristic frequencies $f_{\text{c},i}$, ranging from 2.6 Hz to 2.6 MHz, and amplitudes $F_{0,i}^{1/2}$ as listed in Tab. I(a). For comparison of the fluctuation strengths of the different fluctuators with different $f_{\text{c},i}$, in Tab. I we also list $\Delta\Phi_i = F_{0,i}^{1/2} \cdot \sqrt{2\pi f_{\text{c},i}}$, which yields values in the range $\sim 30\ldots350\,\mu\Phi_0$.

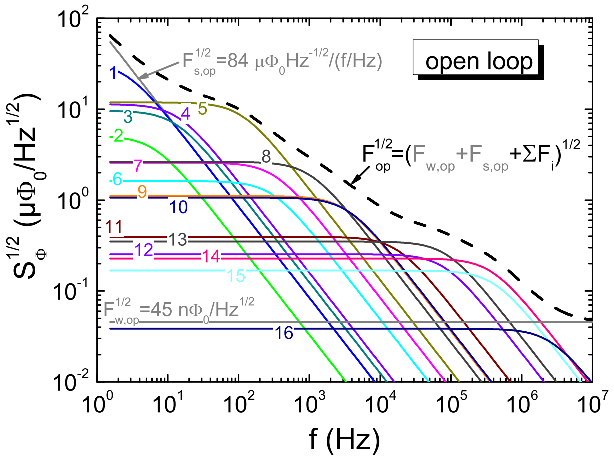


FIG. 4. Analysis of flux noise of SQUID-1: The dashed line is the fit to the noise spectrum, measured open loop (dc bias). This spectrum is the sum of the shown Lorentzians (labeled as $i = 1\ldots16$) plus a white noise contribution plus a $F_s \propto 1/f^2$ contribution.

Figure 5(a) and (b) shows the fits $F_{\text{dc}}^{1/2}(f)$ and $F_{\text{br}}^{1/2}(f)$ to the spectra measured in FLL with dc bias and bias reversal, respectively [cf. Fig. 3(b) in the main text.]. Here, we fixed the white noise contribution in dc bias mode to $F_{\text{w,dc}}^{1/2} = 41\,\text{n}\Phi_0/\text{Hz}^{1/2}$, i.e. a value close to the one obtained for the measurement in open loop mode. The white noise contribution in bias reversal mode is determined by the noise level achieved in dc bias mode at the bias reversal frequency $f_{\text{br}}$, which yields $F_{\text{w,br}}^{1/2} = 231\,\text{n}\Phi_0/\text{Hz}^{1/2}$. The spectrum fitted to the dc bias measurement is decomposed into 15 Lorentzians, while for the bias reversal measurement, fitting with 6 Lorentzians is sufficient. The rms noise at 1 Hz for the bias reversal spectrum is by a factor $\sim 1.8$ lower than the one for the dc bias spectrum. Characteristic frequencies $f_{\text{c},i}$, and amplitudes of the Lorentzians are listed in Tab. I(b) for the dc bias spectrum and in Tab. I(c) for the bias reversal spectrum.

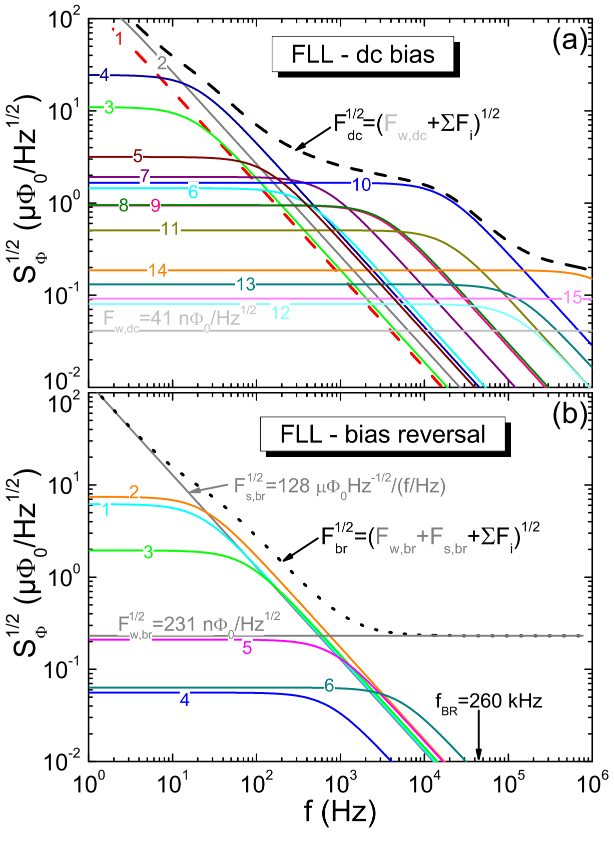

TABLE I. Characteristic frequencies $f_{\mathrm{c},i}$, rms amplitudes $F_{0,i}^{1/2}$ and flux amplitudes $\Delta\Phi_i$ of Lorentzians $F_i$ calculated to approximate the flux noise spectra of SQUID-1, measured (a) in open loop (dc bias) [cf. Fig. 4], (b) in FLL dc bias [cf. Fig. 5(a)], and (c) in FLL bias reversal mode [cf. Fig. 5(b)].

(a) open loop

| $i$ | 1 | 2 | 3 | 4 | 5 | 6 | 7 | 8 | 9 | 10 | 11 | 12 | 13 | 14 | 15 | 16 |
|---|---|---|---|---|---|---|---|---|---|---|---|---|---|---|---|---|
| $f_{\mathrm{c},i}$ (Hz) | 2.6 | 6.5 | 13 | 14 | 111 | 301 | 325 | 1.0 k | 3.3 k | 3.5 k | 18 k | 82 k | 88 k | 380 k | 410 k | 2.6 M |
| $F_{0,i}^{1/2}$ ($\mu\Phi_0/\mathrm{Hz}^{1/2}$) | 33 | 5.1 | 9.6 | 11 | 12 | 1.6 | 2.6 | 2.6 | 1.1 | 1.1 | 0.40 | 0.25 | 0.35 | 0.23 | 0.17 | 0.038 |
| $\Delta\Phi_i$ ($\mu\Phi_0$) | 131 | 32 | 87 | 106 | 314 | 71 | 119 | 211 | 158 | 158 | 131 | 182 | 261 | 352 | 269 | 155 |

(b) FLL – dc bias

| $i$ | 1 | 2 | 3 | 4 | 5 | 6 | 7 | 8 | 9 | 10 | 11 | 12 | 13 | 14 | 15 |
|---|---|---|---|---|---|---|---|---|---|---|---|---|---|---|---|
| $f_{\mathrm{c},i}$ (Hz) | 0.8 | 1 | 17 | 18 | 126 | 369 | 631 | 2.9 k | 3.2 k | 17.1 k | 18.5 k | 117 k | 126 k | 1.4 M | 6.8 M |
| $F_{0,i}^{1/2}$ ($\mu\Phi_0/\mathrm{Hz}^{1/2}$) | 206 | 265 | 11.0 | 24.5 | 3.2 | 1.4 | 1.9 | 0.94 | 0.95 | 1.7 | 0.51 | 0.08 | 0.13 | 0.19 | 0.09 |
| $\Delta\Phi_i$ ($\mu\Phi_0$) | 461 | 665 | 114 | 264 | 89 | 70 | 121 | 128 | 134 | 544 | 173 | 69 | 117 | 546 | 600 |

(c) FLL – bias reversal

| $i$ | 1 | 2 | 3 | 4 | 5 | 6 |
|---|---|---|---|---|---|---|
| $f_{\mathrm{c},i}$ (Hz) | 21 | 23 | 74 | 736 | 794 | 5 k |
| $F_{0,i}^{1/2}$ ($\mu\Phi_0/\mathrm{Hz}^{1/2}$) | 6.2 | 7.4 | 1.9 | 0.056 | 0.21 | 0.063 |
| $\Delta\Phi_i$ ($\mu\Phi_0$) | 72 | 90 | 42 | 3.8 | 15 | 11 |


[1] M. Kemmler, D. Bothner, K. Ilin, M. Siegel, R. Kleiner, and D. Koelle, "Suppression of dissipation in Nb thin films with triangular antidot arrays by random removal of pinning sites," Phys. Rev. B **79**, 184509 (2009).

[2] B. Chesca, R. Kleiner, and D. Koelle, "SQUID Theory," in The SQUD Handbook, Vol. 1: Fundamentals and Technology of SQUIDs and SQUID systems, edited by John Clarke and Alex I. Braginski (Wiley-VCH, Weinheim, 2004) Chap. 2, pp. 29–92.

[3] D. Drung and M. Mück, "SQUID Electronics," in The SQUD Handbook, Vol. 1: Fundamentals and Technology of SQUIDs and SQUID systems, edited by John Clarke and Alex I. Braginski (Wiley-VCH, Weinheim, 2004) Chap. 4, pp. 127–170.

[4] E. Sassier, R. Kleiner, and D. Koelle, "A spectroscopic method for excess-noise spectrum analysis," Unpublished.
